# Supplementary material for: Aspects of Quantum Entanglement and Indistinguishability
Source: arXiv:2503.08623 source file (2025-03-11)
Supplement: Supplementary file 1 [file appa.tex]

\chapter{Tables}

\begin{table}
\caption{Armadillos}
\label{arm:table}
\begin{center}
\begin{tabular}{||l|l||}\hline
Armadillos & are \\\hline
our	   & friends \\\hline
\end{tabular}
\end{center}
\end{table}

\clearpage
\newpage
