# Supplementary material for: Aspects of Quantum Entanglement and Indistinguishability
Source: arXiv:2503.08623 source file (2025-03-11)
Supplement: Supplementary file 2 [file appb.tex]

\chapter{Figures}

\vspace*{-3in}

\begin{figure}
\vspace{2.4in}
\caption{Armadillo slaying lawyer.}
\label{arm:fig1}
\end{figure}
\clearpage
\newpage

\begin{figure}
\vspace{2.4in}
\caption{Armadillo eradicating national debt.}
\label{arm:fig2}
\end{figure}
\clearpage
\newpage
